# Supplementary material for: Schottky barrier lowering due to interface states in 2D heterophase devices
Source: arXiv:1911.09521 source file (2020-10-12)
Supplement: Supplementary file 1 [file Supplementary.pdf]

# Determination of Schottky barriers in 2D heterophase devices.

## Supplementary Material.

Line Jelver<sup>\*1,2</sup>, Daniele Stradi<sup>1</sup>, Kurt Stokbro<sup>1</sup>, and Karsten Wedel Jacobsen<sup>2</sup>

<sup>1</sup>Synopsys Denmark, Fruebjergvej 3, PostBox 4, DK-2100 Copenhagen, Denmark.

<sup>2</sup>Center for Atomic-scale Materials Design (CAMD), Technical University of Denmark, Bldg. 309, DK-2800 Lyngby, Denmark.

November 21, 2019

All calculations have been performed with QuantumATK 2019.03-SP1.<sup>[1]</sup>

## A Substrate effect

The depletion width scales with the effective dielectric constant of the 2D material which is modified by the surrounding dielectric substrate.<sup>[2,3]</sup> The two fabricated MoTe<sub>2</sub> heterophase devices<sup>[4,5]</sup> are both placed on substrates. We therefore investigate the effect of scaling on the depletion width.

Using the Wentzel–Kramers–Brillouin (WKB) approximation and atomic units, the tunneling through an exponential barrier placed at  $x = 0$  with height  $\Phi^{SB}$  and depletion width  $x_D$  is given by,

$$T(E) = e^{-2 \int_0^{x_{cl}} \sqrt{2(V(x)-E)} dx}$$
$$V(x) = \Phi^{SB} e^{-x/x_D}, \quad x > 0$$

Where  $x_{cl}$  is the classical turning point of the barrier. We make the substitution  $z = e^{-x/x_D}$  resulting in,

$$T(E) = e^{-\sqrt{2\Phi^{SB}} x_D \int_{E/\Phi^{SB}}^1 \frac{\sqrt{z-E/\Phi^{SB}}}{z} dz}.$$

Scaling the depletion width by  $s$ ,  $x_D \rightarrow s x_D$ , will therefore result in a transmission,

$$T(E) \rightarrow (T(E))^s$$

---

<sup>\*</sup>jelver@synopsys.com

| scaling   | $T_{I^{TE} > I^{TUN}}$ | $T_{\Phi^{TE} \rightarrow \Phi^{DOS}}$ |
|-----------|------------------------|----------------------------------------|
| 0.5 $x_D$ | 1118 K                 | -                                      |
| 1.0 $x_D$ | 410 K                  | 600 K                                  |
| 1.5 $x_D$ | 236 K                  | 450 K                                  |
| 2.0 $x_D$ | 164 K                  | 250 K                                  |

Table 1: Effect of scaling the depletion width of the n-doped device.

We have scaled the tunneling transmission of the n-doped device using  $s = 0.5$ ,  $s = 1.5$  and  $s = 2$  to investigate the effect of including a substrate. This results in a shift of the two regimes in Figure 4 in the main text. In Table 1, we list the temperature at which the thermionic current becomes larger than the tunneling current,  $T_{I^{TE} > I^{TUN}}$ , and the temperature at which the TE barrier has converged to the value of the DOS barrier,  $T_{\Phi^{TE} \rightarrow \Phi^{DOS}}$ . This shows that the tunneling current remains non-negligible at the relevant temperatures for a depletion width up to twice the size of the calculated width. Note that a scaling factor of 0.5 results in a TE barrier which never converges to the DOS barrier.

## B Setting up the device

The setup and relaxation of the device follows four steps which are illustrated on Figure 1.

1. The 1H and 1T' phases are set up in the conventional unit cell and relaxed to a stress tolerance of 0.1 GPa using periodic boundary conditions. This gives the 2D lattice parameters  $a = 3.59$  Å for the 1H phase and  $a = 3.52$  Å,  $b = 6.34$  Å for the 1T' phase which compares well with the experimental values.<sup>[6,7]</sup>
2. The interface is created using the interface builder in QuantumATK.<sup>[8,9]</sup> The 1T' phase is strained by 2.12 % along the y-direction to make a match between the (100)-face of 1T' and the (01-10)-face of 1H. We choose to strain the 1T' phase in order to maintain the semiconductor properties.
3. A short nanoribbon of this interface is created with 10 atomic layers of each phase and 20 Å of vacuum between periodic images in the x-direction. The 6 atomic layers closest to the interface are allowed to relax and the remaining 1T' phase is fixed while the remaining 1H phase is kept rigid to allow for a compression or elongation of the interface region.
4. The relaxed interface is converted to a device configuration in order to perform the NEGF calculations. The central region is composed of about 5 nm's of 1T' phase and 20 nm's of 1H phase. Each electrode is a single atomic layer of the phase. For these calculation we use Dirichlet boundary conditions between the central region and electrodes, periodic boundary conditions in the y-direction and Neumann boundary conditions in the z-direction to avoid electrostatic interactions between neighbouring interface dipoles.<sup>[10]</sup> The relaxation is performed for the 6 atomic layers closest to the interface of each phase while the rest of the atoms are kept fixed.

## C Joint density of states of the n-doped device

Since we want to compare with the results from the NEGF calculations, which are extended systems, we create purely 1H and purely 1T' phase devices consisting of 4 repetitions of the corresponding electrode in order to calculate the joint density of states.

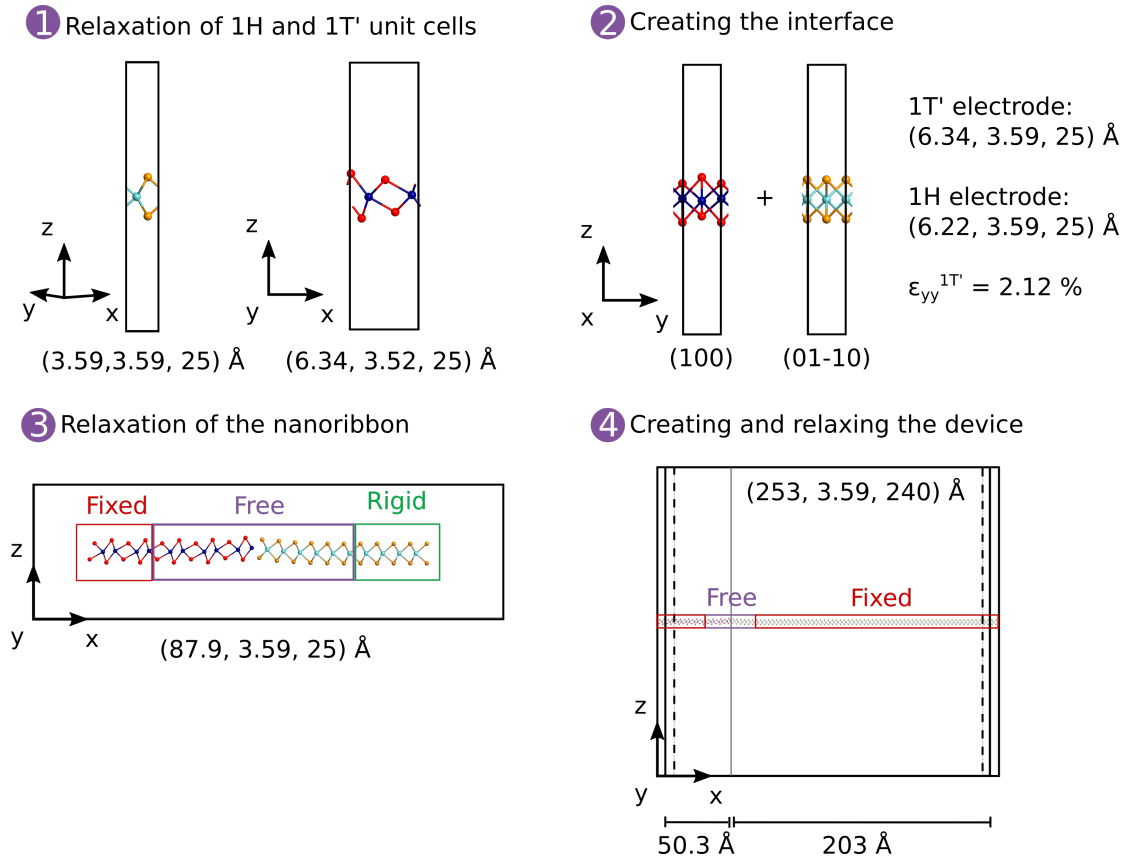

Figure 1: The relaxation scheme for setting up the device along with the unit cells of each calculation.

$$\rho^{L \cap R}(\varepsilon) = \int \rho_L(\varepsilon, k_L) \rho_R(\varepsilon, k_R) \delta(k_L^\perp - k_R^\perp) dk_L dk_R. \quad (\text{C.1})$$

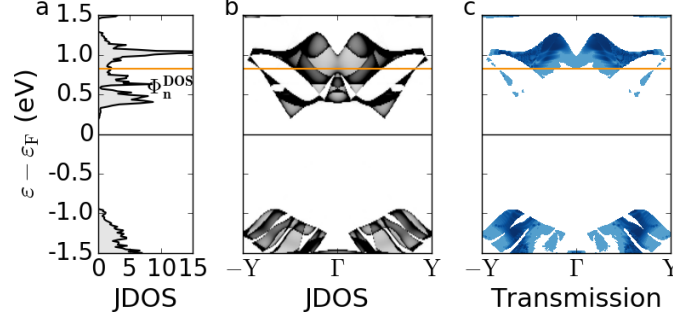

Figure 2: Joint density of states and k-resolved transmission of the n-doped device. **a** shows the JDOS summed over all  $k_y$ -points, **b** shows the k-resolved JDOS, and **c** shows the corresponding k-resolved transmission.

## References

- [1] Søren Smidstrup, Troels Markussen, Pieter Vancraeyveld, Jess Wellendorff, Julian Schneider, Tue Gunst, Brecht Verstichel, Daniele Stradi, Petr A Khomyakov, Ulrik G Vej-Hansen, Maeng-Eun Lee, Samuel T Chill, Filip Rasmussen, Gabriele Penazzi, Fabiano Corsetti, Ari Ojanperä, Kristian Jensen, Mattias L N Palsgaard, Umberto Martinez, Anders Blom, Mads Brandbyge, and Kurt Stokbro. QuantumATK: an integrated platform of electronic and atomic-scale modelling tools. *Journal of Physics: Condensed Matter*, 32(1):015901, 2019. doi: 10.1088/1361-648x/ab4007.
- [2] Henry Yu, Alex Kutana, and Boris I. Yakobson. Carrier Delocalization in Two-Dimensional Coplanar p-n Junctions of Graphene and Metal Dichalcogenides. *Nano Letters*, 16(8):5032–5036, 2016. doi: 10.1021/acs.nanolett.6b01822.
- [3] Ankur Nipane, Sirisha Jayanti, Abhinandan Borah, and James T. Teherani. Electrostatics of lateral p-n junctions in atomically thin materials. *Journal of Applied Physics*, 122(19), 2017. doi: 10.1063/1.4994047.
- [4] Suyeon Cho, S. Kim, J. H. Kim, Jiong Zhao, Jinbong Seok, Dong Hoon Keum, Jaeyoon Baik, D.-H. Choe, K J Chang, Kazu Suenaga, Sung Wng Kim, Young Hee Lee, and Heejun Yang. Phase patterning for ohmic homojunction contact in MoTe2. *Science*, 349(6248):625–628, 2015. doi: 10.1126/science.aab3175.
- [5] Ji Ho Sung, Hoseok Heo, Saerom Si, Yong Hyeon Kim, Hyeong Rae Noh, Kyung Song, Juho Kim, Chang-Soo Lee, Seung-Young Seo, Dong-Hwi Kim, Hyoung Kug Kim, Han Woong Yeom, Tae-Hwan Kim, Si-Young Choi, Jun Sung Kim, and Moon-Ho Jo. Coplanar semiconductor-metal circuitry defined on few-layer MoTe2 via polymorphic heteroepitaxy. *Nature Nanotechnology*, 12:1064, sep 2017.
- [6] Ying Wang, Jun Xiao, Hanyu Zhu, Yao Li, Yousif Alsaied, King Yan Fong, Yao Zhou, Siqi Wang, Wu Shi, Yuan Wang, Alex Zettl, Evan J Reed, and Xiang Zhang. Structural phase transition in monolayer MoTe2 driven by electrostatic doping. *Nature*, 550:487, 2017.
- [7] Carl H. Naylor, William M. Parkin, Jinglei Ping, Zhaoli Gao, Yu Ren Zhou, Youngkuk Kim, Frank Streller, Robert W. Carpick, Andrew M. Rappe, Marija Drndić, James M. Kikkawa, and A. T. Charlie Johnson. Monolayer single-crystal 1T-MoTe 2 grown by chemical vapor deposition exhibits weak antilocalization effect. *Nano Letters*, 16(7):4297–4304, 2016.

- [8] Line Jelver, Peter Mahler Larsen, Daniele Stradi, Kurt Stokbro, and Karsten Wedel Jacobsen. Determination of low-strain interfaces via geometric matching. *Physical Review B*, 96(8):085306, 2017.
- [9] Daniele Stradi, Line Jelver, Søren Smidstrup, and Kurt Stokbro. Method for determining optimal supercell representation of interfaces. *Journal of Physics Condensed Matter*, 29(18), 2017. ISSN 1361648X. doi: 10.1088/1361-648X/aa66f3.
- [10] O. Leenaerts, S. Vercauteren, B. Schoeters, and B. Partoens. System-size dependent band alignment in lateral two-dimensional heterostructures. *2D Materials*, 3(2):025012, 2016.
